# Supplementary material for: Introducing Depth into Transformer-based 3D Object Detection
Source: arXiv:2302.13002 source file (2023-06-05)
Supplement: Supplementary file 1 [file appendix_failure.tex]

\begin{figure*}[tp]
    \centering
    \includegraphics[width=0.9\linewidth]{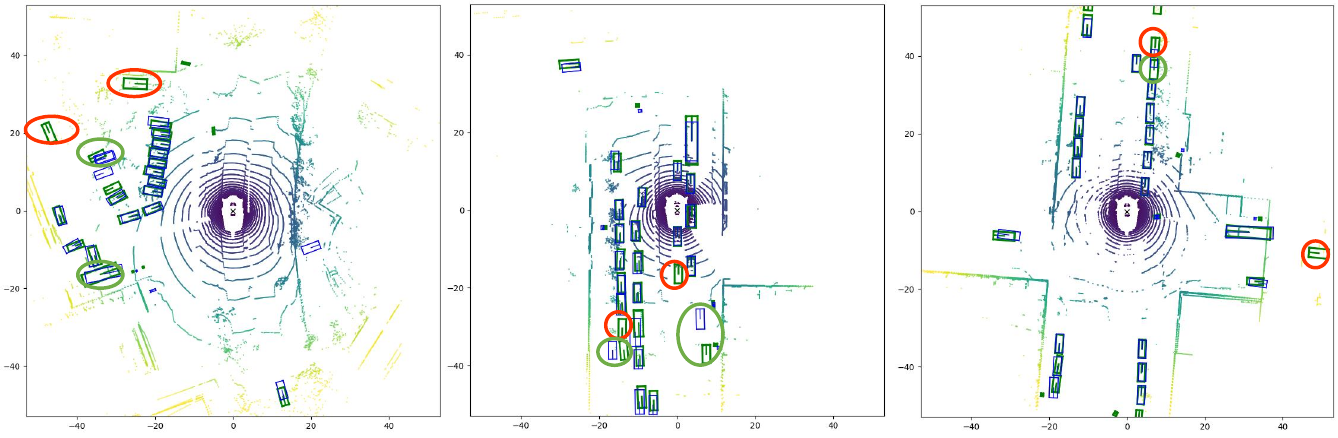}
    \caption{ Some failure cases of \modelname. The green and blue boxes denote GT and predicted boxes, respectively. Green circles represent the prediction is inaccurate because the object is blocked by another object. Red circles mean that the blocked object is undetected.
    }
    \label{fig:appendix vis failure}
\end{figure*}
