# Supplementary material for: Introducing Depth into Transformer-based 3D Object Detection
Source: arXiv:2302.13002 source file (2023-06-05)
Supplement: Supplementary file 2 [file appendix_objectiveness.tex]

\begin{figure*}[tp]
    \centering
    \includegraphics[width=0.9\linewidth]{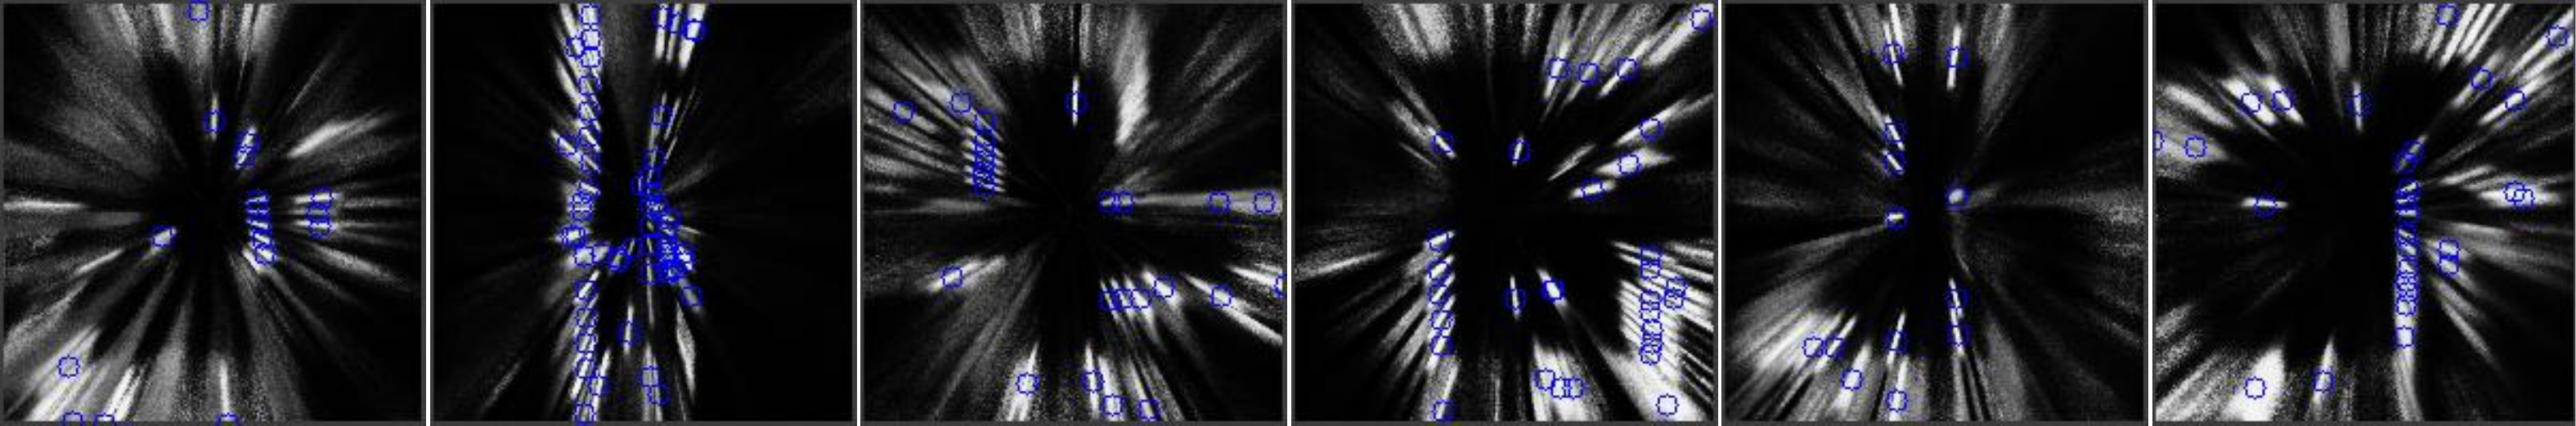}
    \caption{ A visualization of classification scores on BEV. Each blue circle is the center of a GT object. The brightness of a pixel represents the classification scores. The high brightness represents a high classification score.
    }
    \label{fig:appendix vis obj}
\end{figure*}
