# Supplementary material for: Introducing Depth into Transformer-based 3D Object Detection
Source: arXiv:2302.13002 source file (2023-06-05)
Supplement: Supplementary file 3 [file reference_supp.tex]

@String(PAMI = {IEEE Trans. Pattern Anal. Mach. Intell.})
@String(IJCV = {Int. J. Comput. Vis.})
@String(CVPR= {IEEE Conf. Comput. Vis. Pattern Recog.})
@String(ICCV= {Int. Conf. Comput. Vis.})
@String(ECCV= {Eur. Conf. Comput. Vis.})
@String(NIPS= {Adv. Neural Inform. Process. Syst.})
@String(NeurIPS= {Adv. Neural Inform. Process. Syst.})
@String(ICPR = {Int. Conf. Pattern Recog.})
@String(BMVC= {Brit. Mach. Vis. Conf.})
@String(TOG= {ACM Trans. Graph.})
@String(TIP  = {IEEE Trans. Image Process.})
@String(TVCG  = {IEEE Trans. Vis. Comput. Graph.})
@String(TMM  = {IEEE Trans. Multimedia})
@String(ACMMM= {ACM Int. Conf. Multimedia})
@String(ICME = {Int. Conf. Multimedia and Expo})
@String(ICASSP=	{ICASSP})
@String(ICIP = {IEEE Int. Conf. Image Process.})
@String(ACCV  = {ACCV})
@String(ICLR = {Int. Conf. Learn. Represent.})
@String(IJCAI = {IJCAI})
@String(PR   = {Pattern Recognition})
@String(AAAI = {AAAI})
@String(CVPRW= {IEEE Conf. Comput. Vis. Pattern Recog. Worksh.})
@String(CSVT = {IEEE Trans. Circuit Syst. Video Technol.})

@String(SPL	= {IEEE Sign. Process. Letters})
@String(VR   = {Vis. Res.})
@String(JOV	 = {J. Vis.})
@String(TVC  = {The Vis. Comput.})
@String(JCST  = {J. Comput. Sci. Tech.})
@String(CGF  = {Comput. Graph. Forum})
@String(CVM = {Computational Visual Media})

@String(PAMI  = {IEEE TPAMI})
@String(IJCV  = {IJCV})
@String(CVPR  = {CVPR})
@String(ICCV  = {ICCV})
@String(ECCV  = {ECCV})
@String(NIPS  = {NeurIPS})
@String(NeurIPS  = {NeurIPS})
@String(ICPR  = {ICPR})
@String(BMVC  =	{BMVC})
@String(TOG   = {ACM TOG})
@String(TIP   = {IEEE TIP})
@String(TVCG  = {IEEE TVCG})
@String(TCSVT = {IEEE TCSVT})
@String(TMM   =	{IEEE TMM})
@String(ACMMM = {ACM MM})
@String(ICME  =	{ICME})
@String(ICASSP=	{ICASSP})
@String(ICIP  = {ICIP})
@String(ACCV  = {ACCV})
@String(ICLR  = {ICLR})
@String(IJCAI = {IJCAI})
@String(PR = {PR})
@String(AAAI = {AAAI})
@String(CVPRW= {CVPRW})
@String(CSVT = {IEEE TCSVT})
